# Supplementary material for: Pirates of Charity: Exploring Donation-based Abuses in Social Media Platforms
Source: arXiv:2412.15621 source file (2024-12-20)
Supplement: Supplementary file 1 [file appendix_fraud_channels_evaluation.tex]

\section{Assessment of Fraudulent Channels}
\label{sec:fraud_channels_evaluations}

In this section, we provide an assessment of the fraudulent communication channels utilized by scammers in perpetrating donation-based abuses based on the API responses of security risk engines. Specifically, we analyze 225 emails, 136 phone numbers, and 252 URLs. We provide detailed insights for each of these fraud communication channels as below.

\subsection{Evaluation of Fraud Emails}

We conducted a comprehensive evaluation of fraudulent emails across three main categories: (i) creation techniques, (ii) historical age or abuse patterns, and (iii) public reporting of scammer activities. Below, we present further details on our findings.

\BfPara{Email Association and Creation Technique} Through a manual qualitative analysis of 225 fraudulent emails, we found that scammers often create email aliases associated with their websites. Out of these emails, 140 referenced the scamming domain, while the remaining aliases were linked to \emph{Gmail} (83) and \emph{Outlook} (2). The three most popular keywords used by scammers in username creation were \emph{info} (66), \emph{contact} (7), and \emph{admin} (5).

\BfPara{Age} We performed the creation dates analysis of these email analyses and identified that 80\% (180/225) email addresses used in scamming were created within 12 months. The remaining 20\% (45/225) email addresses were created on varying age length: 7 years (23/225), 5 years (2/225), 4 years (3/225), 3 years (5/225), and 2 years (12/225). 

\BfPara{Compromised and Public Reported Accounts} In total, we identified 27 accounts reported by the public as either scamming or compromised. Of these, 5 were reported to anti-phishing entities for abusive behavior, while the remaining 22 were found to be leaked or compromised accounts. We suspect that scammers use compromised accounts for two main purposes: (i) maintaining anonymity, and (ii) launching targeted attacks on the contacts of the compromised accounts.

\subsection{Evaluation of Fraud Phone Numbers}

We perform an analysis of fraudulent phone numbers into three primary areas: (i) the targeted regions for attacks, (ii) public reports concerning the misuse of these phone numbers, and (iii) the preferences of scammers in using phones to perpetrate donation-based abuses. Below, we elaborate further on each of these findings.

\BfPara{Target Region} The fraudulent phone numbers used in donation-based scams were registered across 10 regions. Over 90\% of these numbers were associated with three regions: the ~\emph{US} (100/136), ~\emph{Gambia} (15/136), and ~\emph{Canada} (10/136). 

\BfPara{Public Reported Accounts} Among the reported numbers, we found that 15.44\% (21/136) were publicly reported for various forms of abuse, while 11.76\% (16/136) were involved in activities beyond donation-based scams, such as spamming or phone call solicitations.

\BfPara{Phone Type Preference} Scammers preferred to use three types of phones in their schemes: ~\emph{VOIP} (90/136), ~\emph{landline} (38/136), and ~\emph{toll-free} (8/136). Due to widespread internet support, ~\emph{VOIP} is the most popular choice for scammers. We identified 20 distinct carriers used in the 136 scam numbers, with the top five being ~\emph{Africell} (15), ~\emph{AT\&T} (12), ~\emph{Verizon} (9), ~\emph{Lumen Technologies} (8), and ~\emph{Frontier Communications} (3).

\subsection{Evaluation of Fraud URLs}

To comprehend how scammers initiate targeted attacks via fraud URLs, we analyzed four main categories: (i) the targeted regions for domain registration, (ii) the favored ~\emph{eTLDs}, (iii) the hosting providers used to host websites and (iv) the age duration of the domains. Below, we present detailed insights into each of these aspects.

\BfPara{Registry Region} We identified a total of 32 regions associated with 1,128 scamming domain registrations. Of these, 74.20\% (837/1,128) were registered in the ~\emph{US}. Seven countries—~\emph{Iran} (41), ~\emph{Germany} (40), ~\emph{England} (32), ~\emph{Canada} (26), ~\emph{France} (16), and ~\emph{Russia} (13)—accounted for 14.89\% (168/1,128) of the domains, making them the second most common regions. The remaining 8.51\% (100/1,128) were distributed across 24 other countries, including ~\emph{India}, ~\emph{Australia}, the ~\emph{Netherlands}, and ~\emph{Japan}.

\BfPara{eTLDs} We identified 213 distinct eTLDs used by scammers in domain registrations. Of these, 67.37\% (760/1,128) were comprised in the top five eTLDs: \emph{.com} (420), \emph{.org} (134), \emph{.ly} (131), \emph{.co.uk} (47), and \emph{.net} (28). The remaining eTLDs included \emph{.edu} (15), \emph{.cc} (14), \emph{.me} (13), \emph{.ca} (11), and various others.

\BfPara{Hosting Providers} Among the 186 hosting providers used by scammers to register 1,128 domains, the top five were \emph{Cloud Flare Net} (193), \emph{Amazon 02} (162), \emph{Google Cloud} (147), \emph{Fastly} (55), and \emph{WIX} (42). The remaining providers included \emph{Name Cheap} (23), \emph{Square Space} (20), \emph{Digital Ocean} (17), and others.

\BfPara{Age} We identify that 37.05\% (418/1128) domains were registered in the last 4 years -- 2024 (110/1128), 2023 (186/1128), 2022 (86/118), 2021 (36/1128) and the remaining 62.94\% (710/1128) domains were registered between 2007 to 2020. We suspect scammers prefer to use aged domains in launching attacks compared to newly registered domains to gain organic content evaluation from search engines or potentially evading anti-phishing engines as long-standing benign domains.
